# Supplementary material for: FlashCheck: Exploration of Efficient Evidence Retrieval for Fast Fact-Checking
Source: arXiv:2502.05803 source file (2025-02-16)
Supplement: Supplementary file 1 [file appendix.tex]

\begin{figure}
   \centering
    \includegraphics[width=0.6\linewidth]{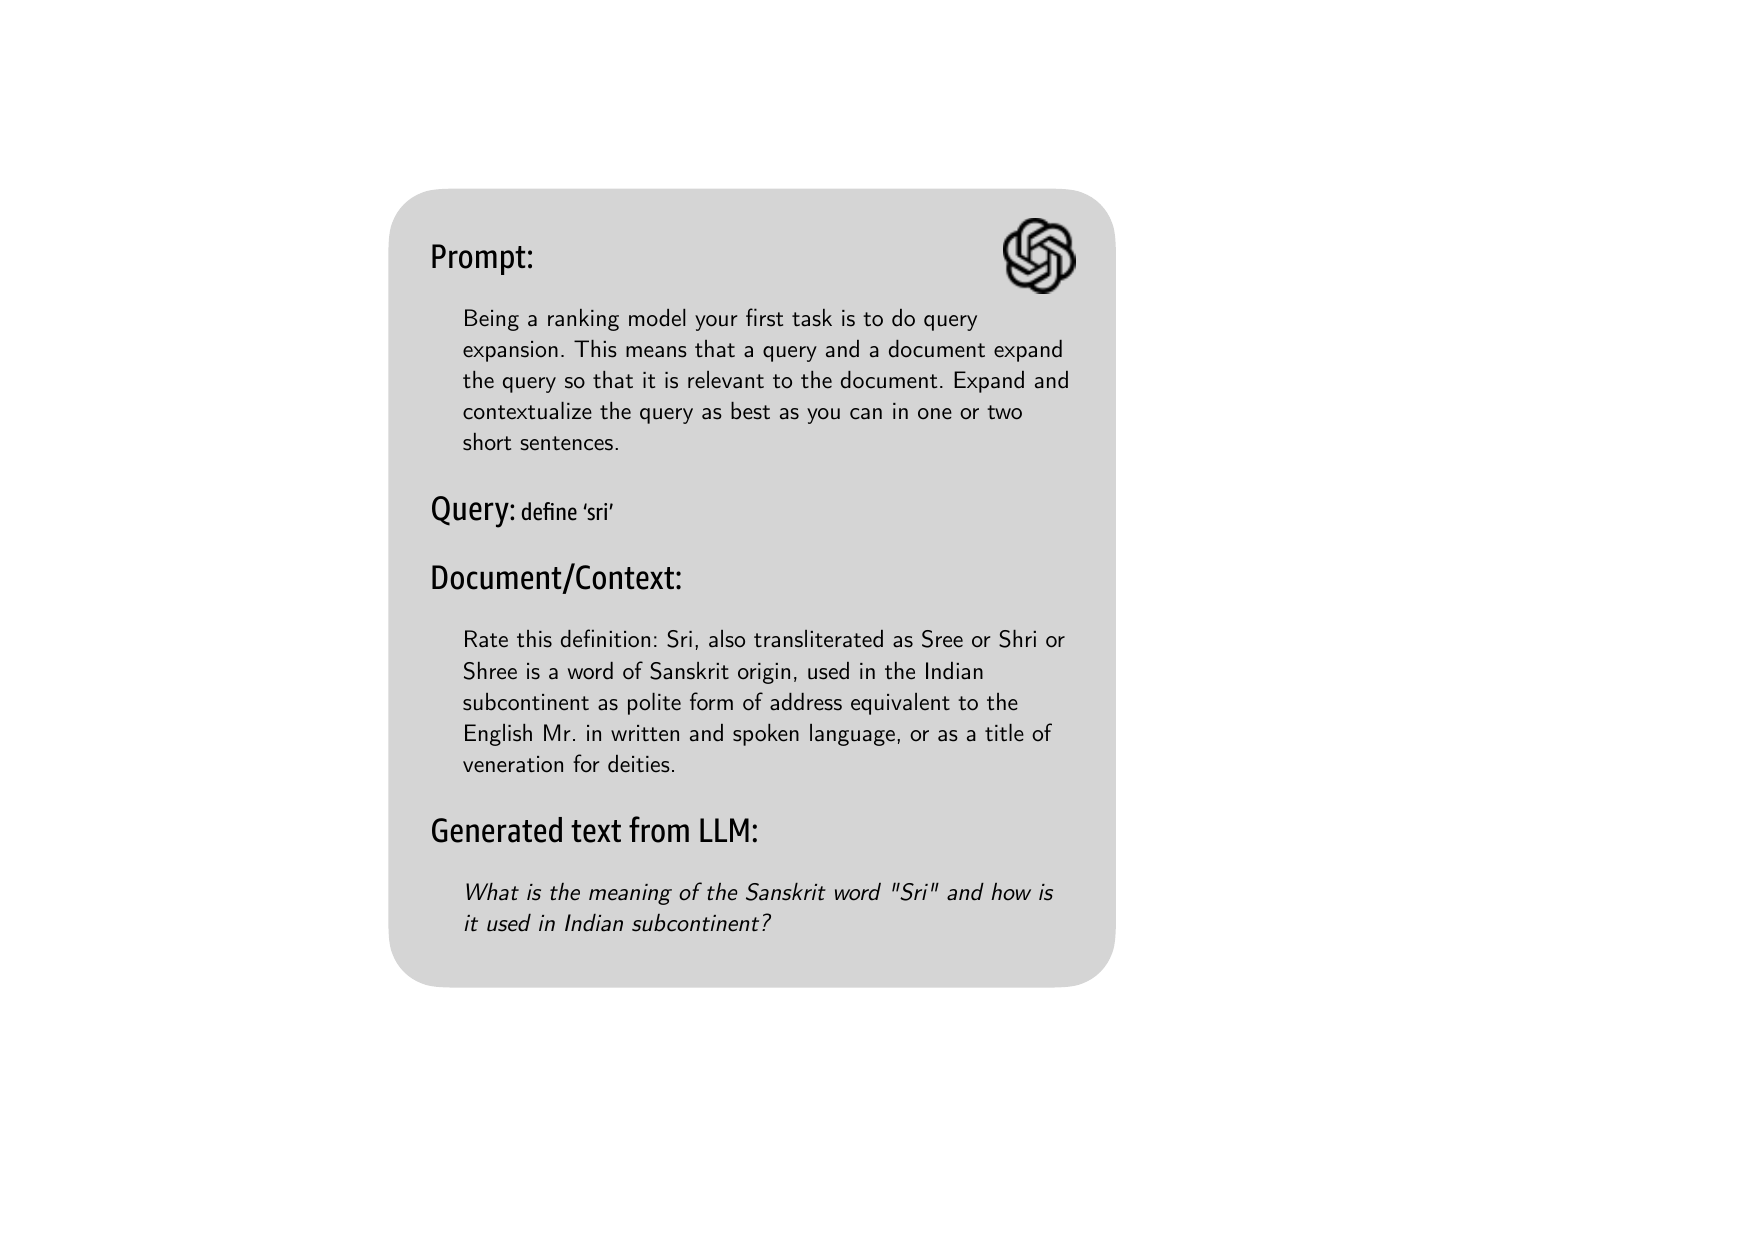}
    \caption{An example of prompting LLM for query rewriting using \car{}.}
   \label{prompting}
\end{figure}

% anecdotal table
%\vspace{-5mm}
\begin{table*}[hbt!]
    \centering
    \begin{tabular}{lccccc}
        \toprule
            \textit{query} & \textit{is\_hard} & \textit{base\_score} & \textit{qpp\_score} & \textit{rank\_fusion} & \textit{qpp\_fusion}\\
            \midrule

eating foods that are considered warm & no & 0.114 & 0.114 & 0.504 & 0.471\\
who was the first steam boat operator & yes & 0.171 & 0.25 & 0.397 & 0.397\\
example of monotonic function & no & 0.180 & 0.180 & 0.247 & 0.283\\
what other brain proteins can cause dementia & no & 0.195 & 0.195 & 0.390 & 0.195\\
causes of military suicide & yes & 0.200 & 0.319 & 0.461 & 0.430\\
does ethambutol treat bone infection & yes & 0.291 & 0.442 & 0.414 & 0.414\\
what is chronometer who invented it & yes & 0.339 & 0.514 & 0.483 & 0.519\\
where are the benefits of cinnamon as a supplement? & yes & 0.346 & 0.559 & 0.637 & 0.559\\
how often to button quail lay eggs & yes & 0.365 & 0.441 & 0.392 & 0.413\\
anthropological definition of environment & no & 0.432 & 0.432 & 0.585 & 0.517\\
how long will methadone stay in your system & no & 0.371 & 0.371 & 0.538 & 0.653\\
how much does it cost to go to alabama university & yes & 0.671 & 0.704 & 0.704 & 0.704\\
what drives poaching & yes & 0.503 & 0.728 & 0.518 & 0.706\\
causes of gas in large intestine & no & 0.236 & 0.236 & 0.631 & 0.541\\
why does lacquered brass tarnish & yes & 0.578 & 0.684 & 0.686 & 0.765\\

        \bottomrule        
    \end{tabular}
    \caption{Comparing nDCG@10 scores for all approaches at query level. The queries are from \mshard{} document collection re-written using \chatgpt{} and \car{} method}
    \vspace{-5mm}
    \label{tab:compare_all_approaches}
\end{table*}

\begin{table*}
\begin{tabular}{lp{.82\textwidth}}
\toprule
    \textbf{Method}     & \textbf{Query Text} \\
\midrule
\textbf{Original query}  & \textbf{define sri}\\
\qd{}  & SRI stands for "Stanford Research Institute," which is a nonprofit research organization that was founded in 1946 as part of Stanford University. Over the years, SRI has conducted groundbreaking research in a wide range [\dots] \\
\vinci{}  & Sri is a Sanskrit word meaning “holy” or “auspicious.” It is often used in Hinduism as an honorific title for a deity or spiritual teacher. It is also used in Buddhist and Jain contexts, and is an important concept in South Asian culture. \\
\chatgpt{}  & Find the definition and meaning of the acronym SRI (Socially Responsible Investing).\\
\car (\vinci{})  & What is the meaning of Sanskrit word "Sri" and how is it used as a title of veneration? \\
\car (\chatgpt{})  & What is the meaning of the Sanskrit word "Sri" and how is it used in Indian subcontinent?\\
% \car (\vinci{})(doc)  & What is the origin and meaning of the term "Sri"? \\
% \car (\chatgpt{})(doc)  & What is the origin of the word "Sri" used in India and other South Asian countries?\\
\midrule
\midrule

\textbf{Original query}  & \textbf{hs worms}\\
\qd{}  & HS Worms can refer to several different things depending on the context. If you are referring to HS Worms as an educational institution, then it stands for Hochschule Worms which is a university of applied sciences or it can refer to heartworms [\dots] \\
\vinci{}  & Find information about heartworms in dogs\\
\chatgpt{}  & Find information about the symptoms, causes, and treatment options for heartworm disease in dogs (also known as HS worms).\\
\car (\vinci{})  & What are the courses offered by Hochschule Worms?\\
\car (\chatgpt{})  & What are the programs offered by Hochschule Worms?\\
% \car (\vinci{})(doc)  & What is the country rank and world rank of HS Worms University?\\
% \car (\chatgpt{})(doc)  & What is Hochschule Worms (HS Worms) and where is it located?\\
\midrule
\midrule

\textbf{Original query}  & \textbf{ephesians 6:5-9}\\
\qd{}  & Ephesians 6:5-9 is a passage from the New Testament that speaks to the relationship between slaves and masters in ancient times. It begins by instructing slaves to obey their earthly masters with respect [\dots] \\
\vinci{}  & Find information about Ephesians 6:5-9.\\
\chatgpt{}  & What is the meaning and interpretation of Ephesians 6:5-9 in the Bible?\\
\car (\vinci{})  & 7 With good will render service, as to the Lord, and not to men, 8 knowing that whatever good thing each one does, this he will receive back from the Lord\\
\car (\chatgpt{})  & How does the passage in Ephesians 6:5-9 instruct slaves to behave towards their masters?\\
% \car (\vinci{})(doc)  & too have a Master in heaven. What does Ephesians 6:5-9 teach about the relationship between slaves and masters? \\
% \car (\chatgpt{})(doc)  & What is the meaning of Ephesians 6:5-9 in relation to submission and slavery?\\
\midrule
\midrule

\textbf{Original query}   & \textbf{price nrz}\\
\qd{}  & Price NRZ stands for "Non-Return-to-Zero" and refers to a digital signal encoding technique used in telecommunications. In this technique, the voltage level of the signal remains constant during each bit interval[\dots] \\
\vinci{}  & Find information on the Pricing of Non-Recourse Z-Bonds.\\
\chatgpt{}  & Find information on the pricing strategy for non-return-to-zero (NRZ) encoding.\\
\car (\vinci{})  & What is the pricing of New Residential Investment Corp. common stock on Jan 30, 2017 7:16 PM EST?\\
\car (\chatgpt{})  & What is the public offering price of New Residential Investment Corp.'s common stock?\\
% \car (\vinci{})(doc)  & announced today that it has entered into definitive agreements to acquire Shellpoint Partners, LLC ("Shellpoint"), a leading mortgage servicer and originator.hat is the price of New Residential Investment Corp (NRZ) stock \\
% \car (\chatgpt{})(doc)  & What is the current share price and financial information of New Residential Investment Corp (NRZ)?\\
\midrule

\end{tabular}
\caption{Comparing \textbf{Original} ambiguous queries with their rewrites using \qd{}, \vinci{}, \chatgpt{} approach with in-context and context aware rewriter(\car{}) techniques.}
% Approach with \textbf{(doc)} are rewrites using \ms{} document corpus and the rest from \ms{} passage corpus.
\label{tab:anecdotal_or}
\vspace{-0.25cm}
\end{table*}

\begin{algorithm}[t]
     \DontPrintSemicolon
     \SetKwFunction{Rewrite}{rewrite}
                 \tcp{Training Phase}

     \SetKw{In}{in}
     \KwIn{training batch $D$}
     \KwOut{training batch with rewritten queries $D'$}
     $D' \leftarrow$ empty list\;

     \ForEach{$(q, d^+)$ \In $D$}{
         \tcp{create rewritten query}
         $q^* \leftarrow RE(q,d^+)$\;
         append $(q^*, d^+)$ to $D'$\;
         Fine-tune ranker on $D'$
     }
     \Return{$D'$} \\
                 \tcp{Inference Phase}
             \SetKw{In}{in}
     \KwIn{test set $D_t$}
     \KwOut{Ranked documents}
                \ForEach{$(q_t,d)$ \In $D_t$}{
                $\hat{y} \gets (q_t,d)$
 } 
     \caption{Query Rewriting, Fine-tuning and Ranking}
     \label{alg:augmentation}
    
 \end{algorithm}
